# Supplementary material for: Elasticity Detection: A Building Block for Internet Congestion Control
Source: arXiv:1802.08730 source file (2020-02-15)
Supplement: Supplementary file 1 [file realworld-appendix.tex]

\section{Real Internet Paths}
\label{app:realworld}

We tested \name on $18$ paths in total; we report the mean throughput and delay each protocol achieved on each path in \Fig{full-realworld}.
%
%Overall, \possname performance is comparable to that of other state-of-the-art protocols.

\begin{figure*}
    \centering
    \begin{subfigure}[b]{0.33\textwidth}
        \includegraphics[width=\textwidth]{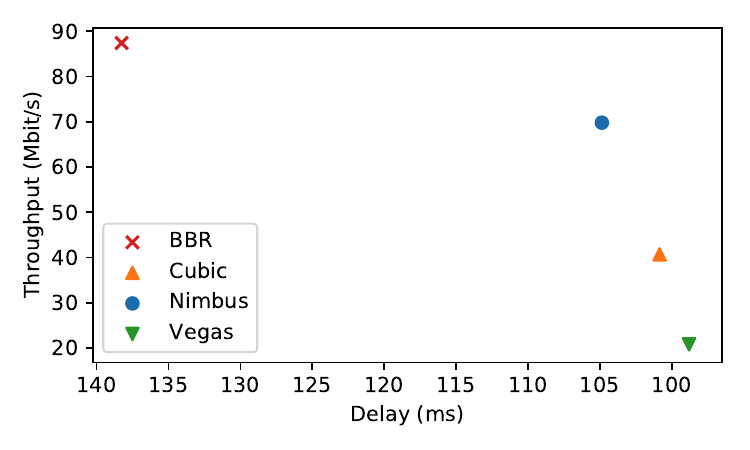}
        \caption{EC2 London -- Host A}
        \label{fig:realworld:london:A}
    \end{subfigure}
    \begin{subfigure}[b]{0.33\textwidth}
        \includegraphics[width=\textwidth]{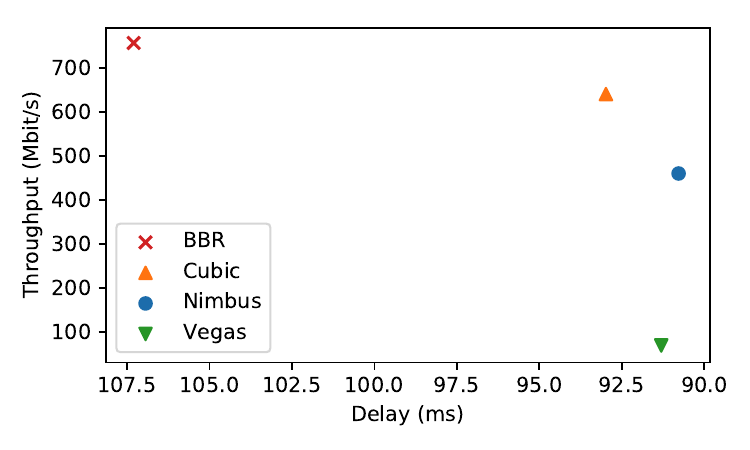}
        \caption{EC2 London -- Host B}
        \label{fig:realworld:london:B}
    \end{subfigure}
    \begin{subfigure}[b]{0.33\textwidth}
        \includegraphics[width=\textwidth]{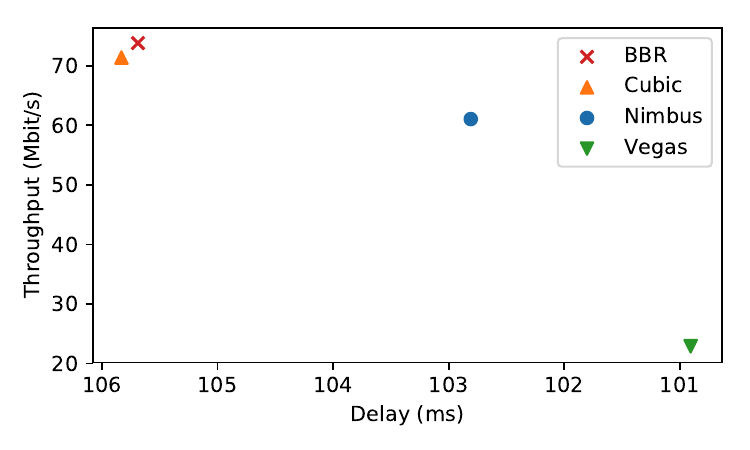}
        \caption{EC2 London -- Host C}
        \label{fig:realworld:london:C}
    \end{subfigure}
    \\
    \begin{subfigure}[b]{0.33\textwidth}
        \includegraphics[width=\textwidth]{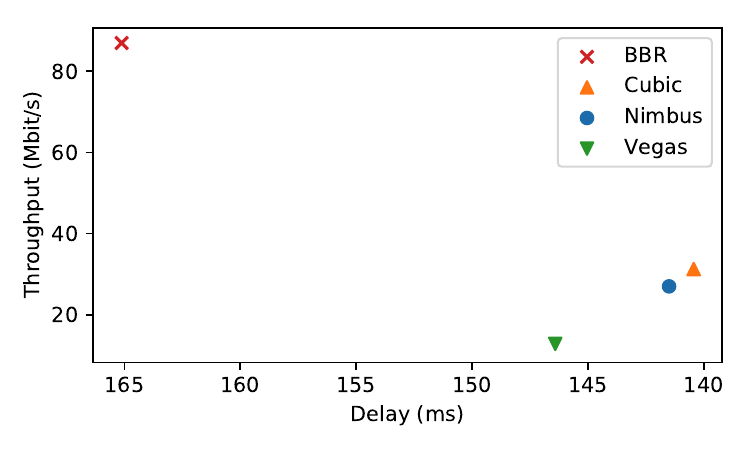}
        \caption{EC2 Brazil -- Host A}
        \label{fig:realworld:brazil:A}
    \end{subfigure}
    \begin{subfigure}[b]{0.33\textwidth}
        \includegraphics[width=\textwidth]{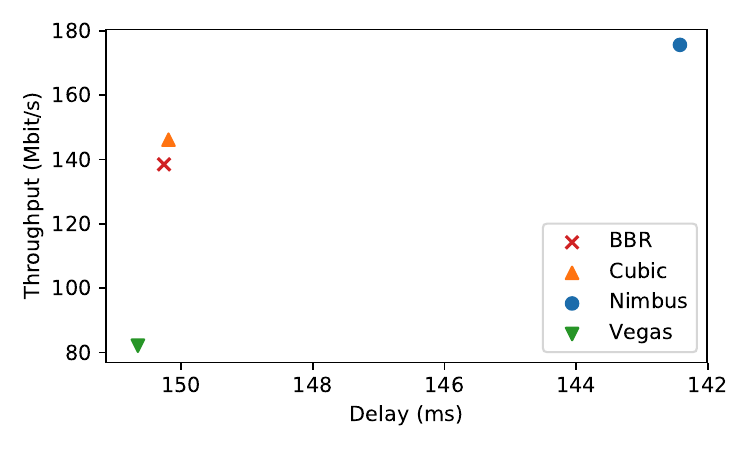}
        \caption{EC2 Brazil -- Host B}
        \label{fig:realworld:brazil:B}
    \end{subfigure}
    \begin{subfigure}[b]{0.33\textwidth}
        \includegraphics[width=\textwidth]{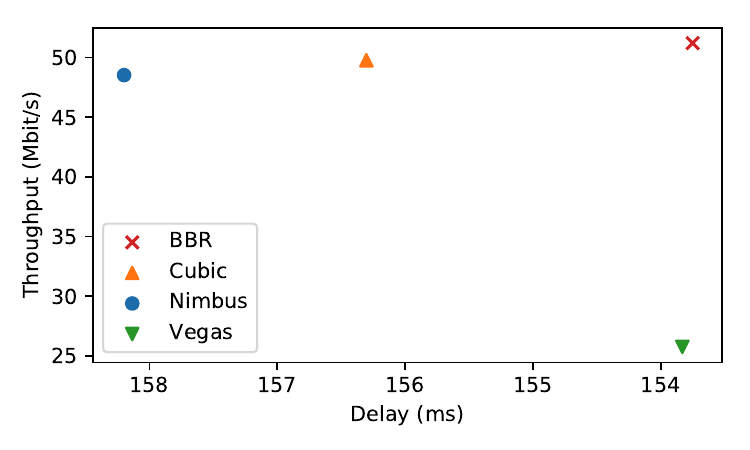}
        \caption{EC2 Brazil -- Host C}
        \label{fig:realworld:brazil:C}
    \end{subfigure}
    \\
    \begin{subfigure}[b]{0.33\textwidth}
        \includegraphics[width=\textwidth]{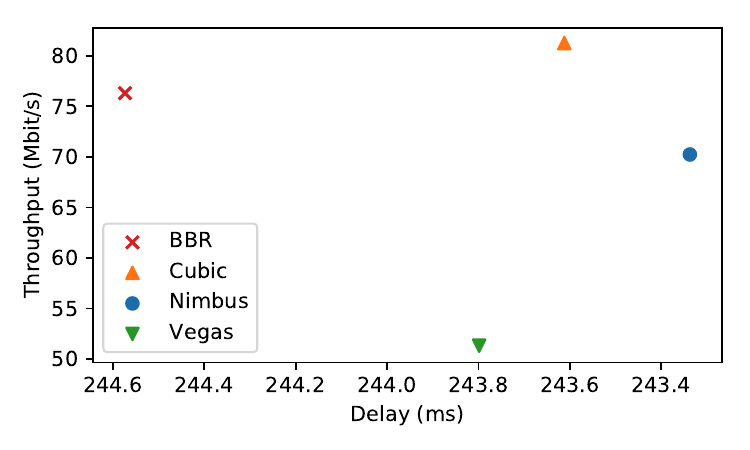}
        \caption{EC2 Sydney -- Host A}
        \label{fig:realworld:sydney:A}
    \end{subfigure}
    \begin{subfigure}[b]{0.33\textwidth}
        \includegraphics[width=\textwidth]{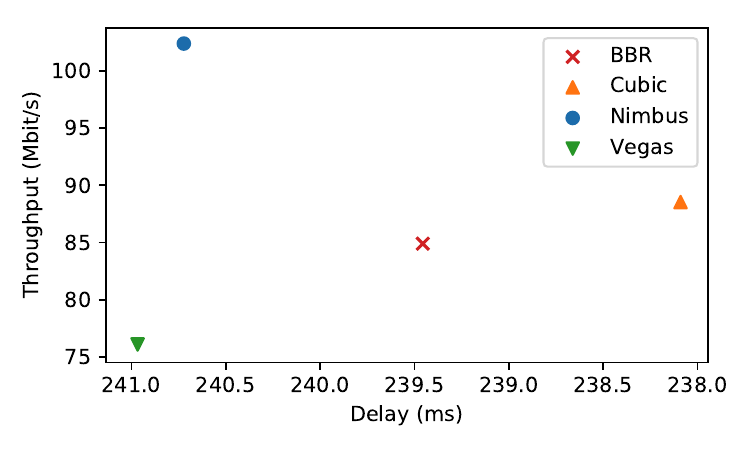}
        \caption{EC2 Sydney -- Host B}
        \label{fig:realworld:sydney:B}
    \end{subfigure}
    \begin{subfigure}[b]{0.33\textwidth}
        \includegraphics[width=\textwidth]{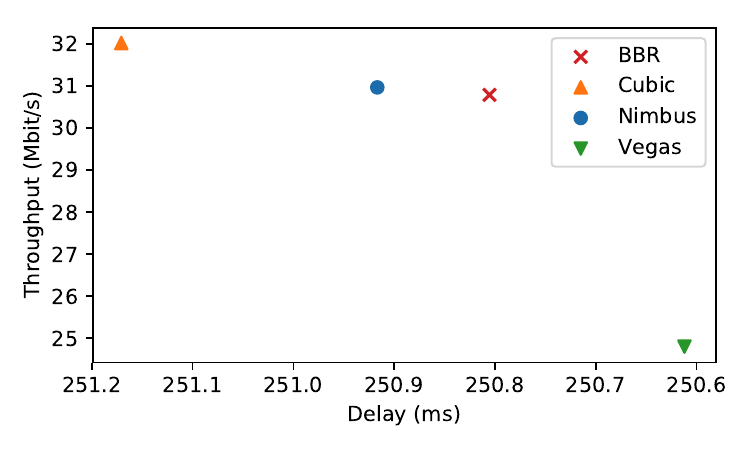}
        \caption{EC2 Sydney -- Host C}
        \label{fig:realworld:sydney:C}
    \end{subfigure}
    \\
    \begin{subfigure}[b]{0.33\textwidth}
        \includegraphics[width=\textwidth]{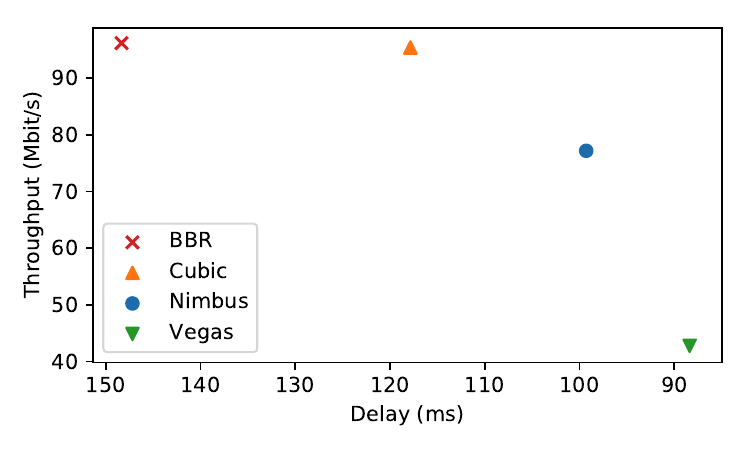}
        \caption{EC2 California -- Host A}
        \label{fig:realworld:california:A}
    \end{subfigure}
    \begin{subfigure}[b]{0.33\textwidth}
        \includegraphics[width=\textwidth]{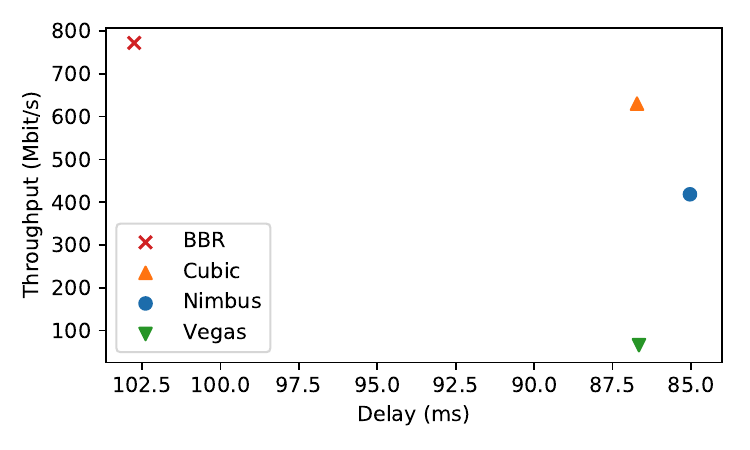}
        \caption{EC2 California -- Host B}
        \label{fig:realworld:california:B}
    \end{subfigure}
    \begin{subfigure}[b]{0.33\textwidth}
        \includegraphics[width=\textwidth]{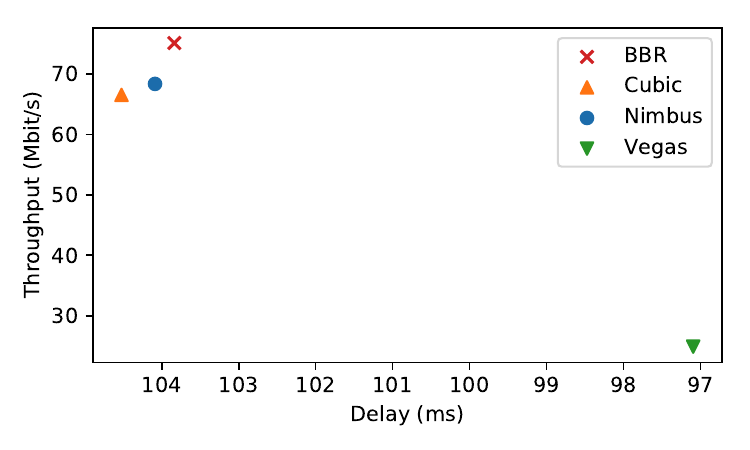}
        \caption{EC2 California -- Host C}
        \label{fig:realworld:california:C}
    \end{subfigure}
    \\
    \begin{subfigure}[b]{0.33\textwidth}
        \includegraphics[width=\textwidth]{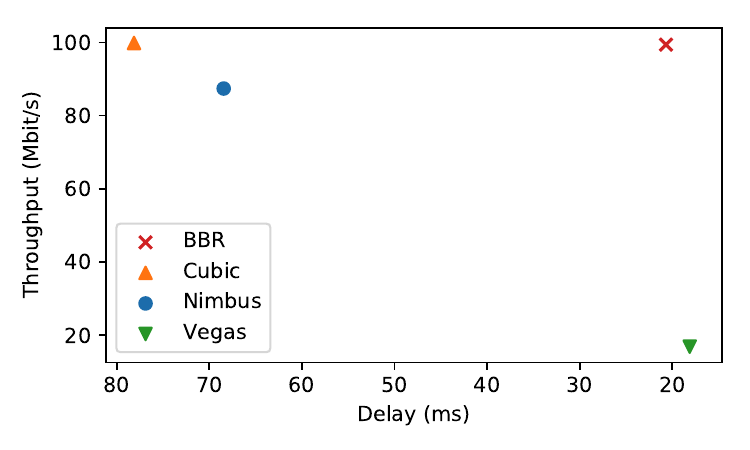}
        \caption{EC2 University -- Host A}
        \label{fig:realworld:univ:A}
    \end{subfigure}
    \begin{subfigure}[b]{0.33\textwidth}
        \includegraphics[width=\textwidth]{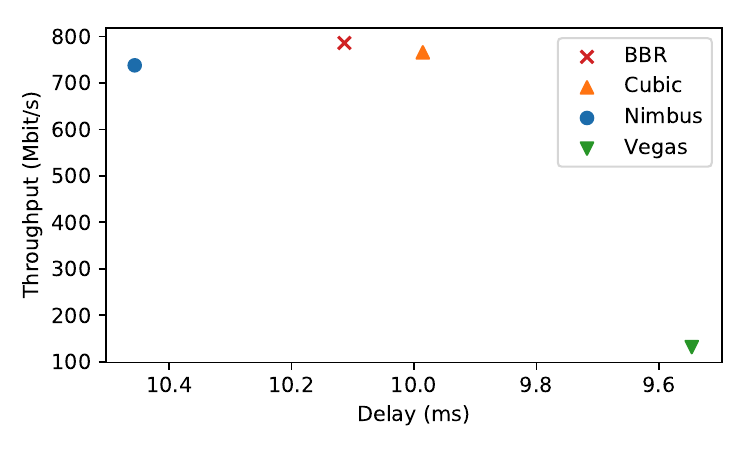}
        \caption{EC2 University -- Host B}
        \label{fig:realworld:univ:B}
    \end{subfigure}
    \begin{subfigure}[b]{0.33\textwidth}
        \includegraphics[width=\textwidth]{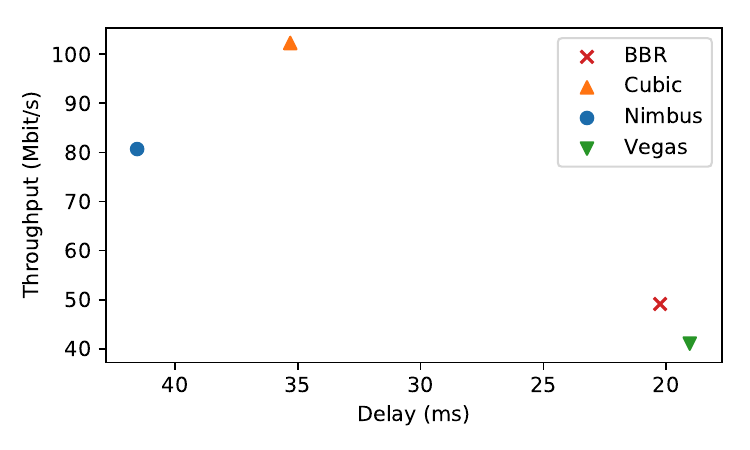}
        \caption{EC2 University -- Host C}
        \label{fig:realworld:univ:C}
    \end{subfigure}
    \caption{\small {\bf Evaluation on Internet paths}---Throughput and latency performance for BBR, Cubic, \name, and Vegas on 18 Internet paths spanning 6 EC2 instances across 5 continents.}
    \label{fig:full-realworld}
\end{figure*}
