# Supplementary material for: Elasticity Detection: A Building Block for Internet Congestion Control
Source: arXiv:1802.08730 source file (2020-02-15)
Supplement: Supplementary file 2 [file related-appendix.tex]

\section{Related Work}
\label{app:related}

Vegas aims to maintain between $\alpha$ and $\beta$ packets in the bottleneck queue using AIAD on its window. 
%% \name allows the endpoint to set a threshold delay,
%% and uses both the current delay and the change in delays as signals to stay
%% close to this target delay.
Fast TCP\cite{fasttcp} exploits delay information to  set its congestion window to maintain a fixed number of packets in the bottleneck queue. While this goal is similar to Vegas, FAST is tuned for higher rates.
TCP Nice~\cite{tcp-nice} and LEDBAT~\cite{rfc6817} are delay-based algorithms to utilize spare
bandwidth without hurting ``foreground'' transfers like web traffic. These schemes don't perform well competing with buffer-filling algorithms.

\if 0

Nice
maintains two estimates of RTTs, a min RTT and a max RTT, through which it
tracks an estimate of the maximum queueing delay possible. Along with Vegas-like
increase/decrease rules, Nice multiplicatively decreases its congestion window
whenever a fraction $f$ of its packets experience queueing delay more than a
fraction $t$ of the maximum queueing delay possible. LEDBAT~\cite{rfc6817} is
another delay-based algorithm with a set target delay. It increases its
congestion window proportional to the difference between the target and the
current delay, \ie target - current.

FAST, Nice and LEDBAT can achieve high throughput and low delays when there is a
low volume of cross-traffic. But they are not designed to be
throughput-competitive with loss-based algorithms that probe aggressively for
bandwidth. \name detects the presence of aggressive cross-traffic, and competes
fairly by switching to its TCP-competitive mode.

\fi

Compound TCP~\cite{compound} maintains both a loss-based window and
a delay-based window, and transmits data based on the sum of the two
windows. The delay-based window is updated with rules similar to Vegas. Compound
achieves high throughput as soon as the link utilization drops, because of its
delay window, but does not control delays because of its loss window.

%%mPERT~\cite{mpert} \ngs{Should complete this.}
%%% Prateesh on mPERT:
%%% http://www.hamilton.ie/lukasz/downloads/papers/IWQoS-draft-08.pdf They have
%%% designed an algorithm where drop_probability is virtually set as a function
%%% of current queuing delay, For a particular Throughput (or drop probability)
%%% there are two points(or
%%% queuing delays), one with low queuing delay and one with high queuing delay,
%%% In absence of elastic background traffic the equilibrium happens at low
%%% queuing delay, in presence of elastic queueing traffic the equilibrium is at
%%% higher queuing delay

\if 0

Equation-based congestion control
(EBCC~\cite{ebcc}) sends traffic at a rate computed to match TCP under similar
RTT and drop probabilities in the network.  EBCC maintains a rate of `loss
events,' where a loss event may include multiple packets lost within an RTT. The
loss event rate and the RTT are used to compute the desired transmission rate
using the TCP throughput equation. EBCC uses packet loss as a signal for
congestion control, and hence cannot achieve a low queueing delay. In contrast,
\name controls delays directly.

MulTCP~\cite{multcp} emulates the behavior of an aggregate of $N$ TCP loss-based
algorithms. It evolves its congestion window as follows. It increases its
congestion window by $N/cwnd$ for each ACK, and decreases it to $cwnd *
(N-0.5)/N$ after each drop. However, as our experiments show (\S\ref{s:eval}),
MulTCP sending rates are very bursty and variable, and MulTCP competes unfairly
with other loss-based TCPs. \name's TCP-competitive mode is smoother and fairer
to other elastic traffic than MulTCP.

\fi

BBR~\cite{bbr} maintains estimates of the bottleneck bandwidth ($b$) and minimum
propagation delay ($d$). The bandwidth estimate tracks the maximum packet
delivery rate to the receiver, while the delay estimate tracks the minimum delay
achieved. BBR paces traffic at a rate $b$ keeping $b * d$ packets in flight.
Unfortunately, the presence of other loss-based algorithms sharing the
bottleneck buffer inflates BBR's delay estimate $d$. Depending on the bottleneck
buffer size, either the BBR-induced losses limit the throughput of the
other TCP flows, or BBR's delay probing reduces its in-flight data, resulting in
lower throughput for BBR itself~\cite{bbr-reno-graph}.

\if 0
We believe both
scenarios are undesirable. In contrast, \name competes fairly by detecting the
presence of other elastic traffic through a novel elasticity detector, and
switches to TCP-competitive mode.

\fi

\if 0

Switch-based algorithms like XCP~\cite{xcp}, RCP~\cite{rcp} and PIE~\cite{pie}
employ feedback loops much similar to \name's delay mode, using spare bandwidth
and queueing delay to control endpoint sending rates. In contrast, \name delay
mode applies this control end-to-end by estimating the spare bandwidth through
the derivative of the queueing delay. This estimation requires us to retain
nonzero queueing delays; this is anyway beneficial to maintain high utilization.

\fi
