# Supplementary material for: Elasticity Detection: A Building Block for Internet Congestion Control
Source: arXiv:1802.08730 source file (2020-02-15)
Supplement: Supplementary file 3 [file switching-robustness-appendix.tex]

\section{Robustness of Switching}
\label{app:switch-robust}
\begin{figure}[t]
    \centering
    \begin{subfigure}[b]{0.4\textwidth}
        \includegraphics[width=\textwidth]{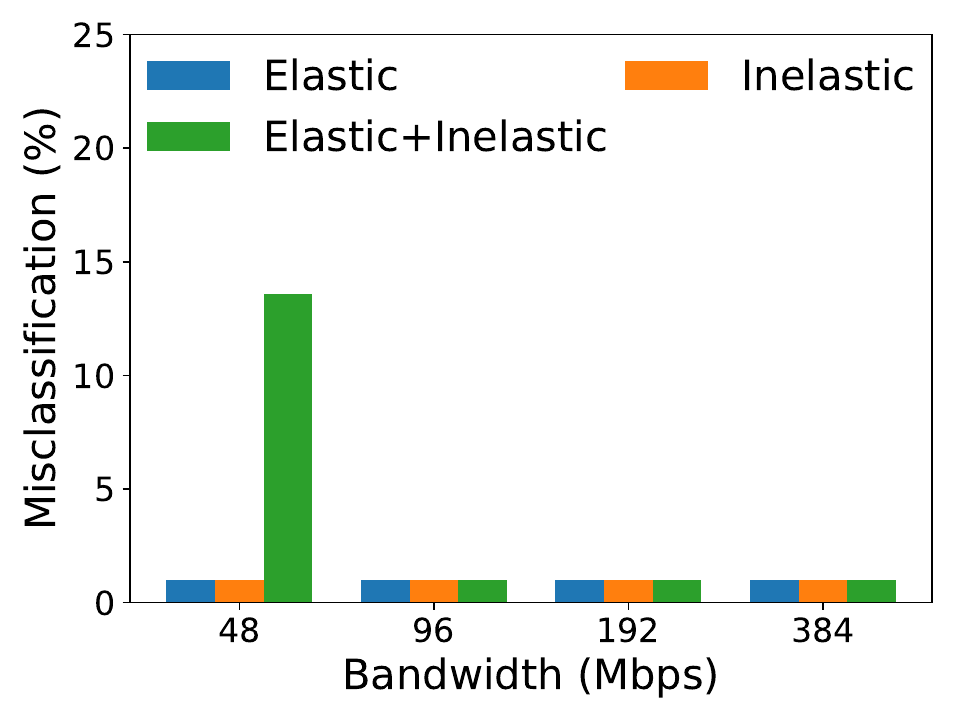}
        \caption{Bandwidth}
        \label{fig::robustness:reno}
    \end{subfigure}
    \begin{subfigure}[b]{0.4\textwidth}
        \includegraphics[width=\textwidth]{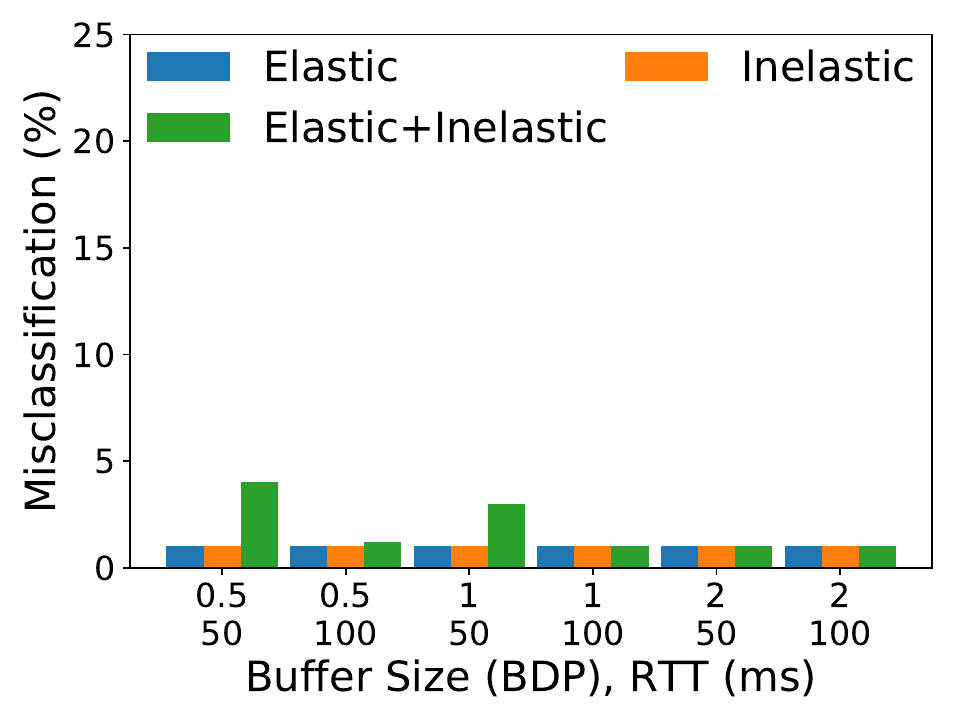}
        \caption{Buffer Size and RTT}
        \label{fig:robustness:buffer_rtt}
    \end{subfigure}
    \begin{subfigure}[b]{0.4\textwidth}
        \includegraphics[width=\textwidth]{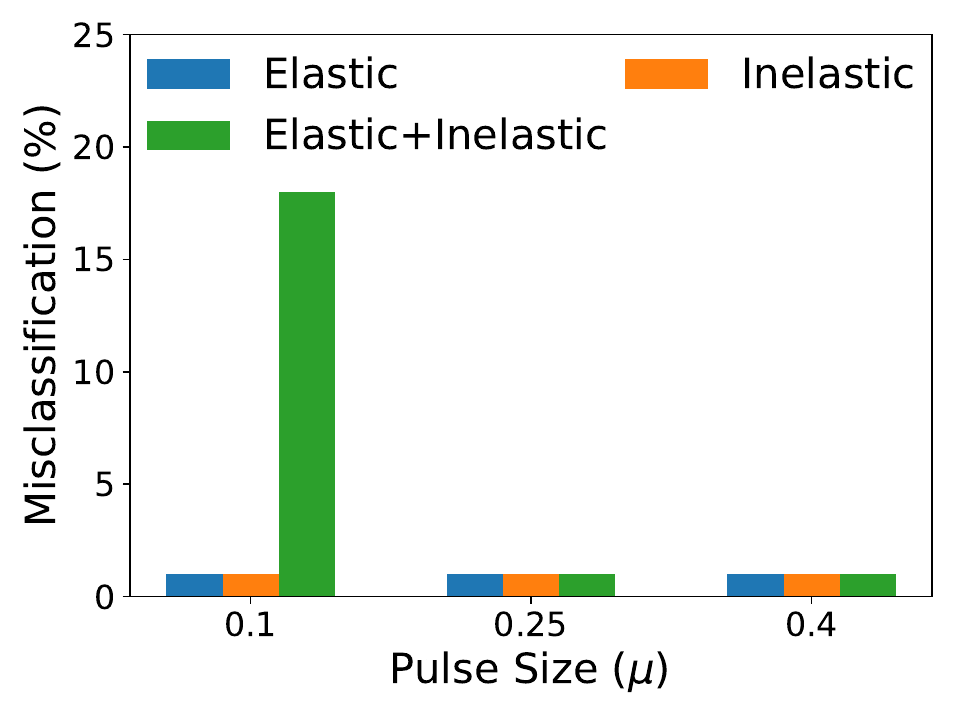}
        \caption{Pulse Size}
        \label{fig:robustness:pulse_size}
    \end{subfigure} 
    \begin{subfigure}[b]{0.4\textwidth}
        \includegraphics[width=\columnwidth]{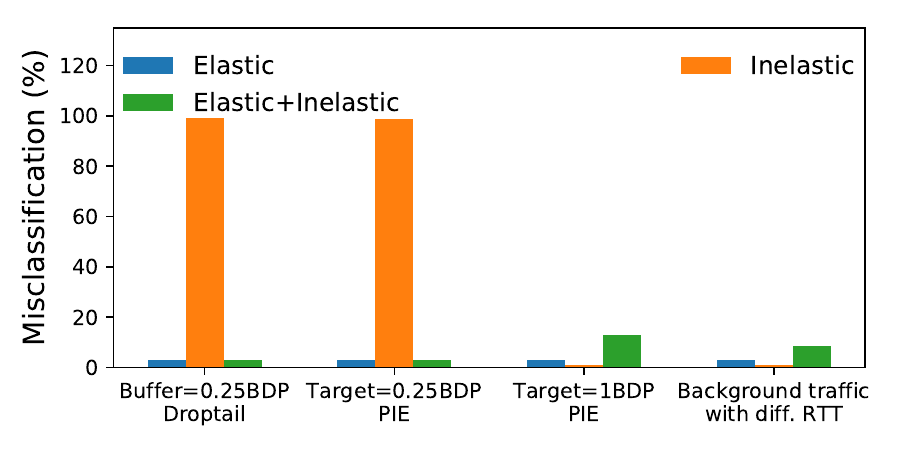}
        \caption{Switching with shallow buffers and AQM.}
        \label{fig:aqm-robustness}
    \end{subfigure}
    \caption{\small {\bf Robustness of switching---}across different values of bandwidth, buffer size and RTTs, pulse size, and active queue management schemes.}
    \label{fig:robustness}
\end{figure}

\Fig{robustness} shows the fraction of time spent in the incorrect mode, or the mis-classification rate, for various network conditions.
\Fig{aqm-robustness} shows the same metric when using small buffers and a number of active queue management schemes.

\name works well for classes Elastic and Inelastic but makes some classification error for Elastic+Inelastic. 
Switching works better in cases where the pulse size is bigger than the standard deviation of background traffic. 
When pulse size is small, this condition might break and \name can make errors in classification. 
On low bandwidth links the standard deviation in background traffic become comparable to pulse size leading to mis-classification.
