# Supplementary material for: Elasticity Detection: A Building Block for Internet Congestion Control
Source: arXiv:1802.08730 source file (2020-02-15)
Supplement: Supplementary file 4 [file appendix.tex]

\section{Is Cross Traffic Ever Inelastic?}
\label{app:delay-control-motivation}

Our experiments on more than 25 Internet paths show that scenarios where cross traffic is predominantly inelastic are common. Figure~\ref{fig:dsmotivation} shows the average throughput and delay for 100 runs of a buffer-filling scheme (Cubic) compared to a delay-based scheme (BasicDelay, described in $\S$\ref{s:nimbus-protocol}) on one of these paths. The \dcc scheme generally achieves much lower delays than Cubic, with similar throughput. This shows that there is an opportunity to significantly improve delays using \dcc algorithms, provided we can detect loss-based TCPs and compete with them fairly when needed. 

\begin{figure}[tbh]
    \includegraphics[width=\columnwidth]{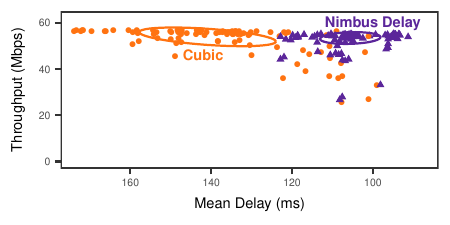}
    \caption{\small \textbf{Loss-based vs. delay-based congestion control.}  The plot shows the average throughput and delay for 100 experiments with Cubic and the Nimbus delay-control algorithm (\S\ref{s:nimbus-protocol}). The experiments were run between a residential client (location redacted for anonymity) and an EC2 server in California. Each experiment lasted one minute.}
    \label{fig:dsmotivation}
    \vspace*{-3pt}
\end{figure}

\section{Does Mode Switching Help Cross-Traffic?}
\label{app:cross-traffic-impact}

\begin{figure}[t]
    \centering
    \includegraphics[width=0.48\textwidth]{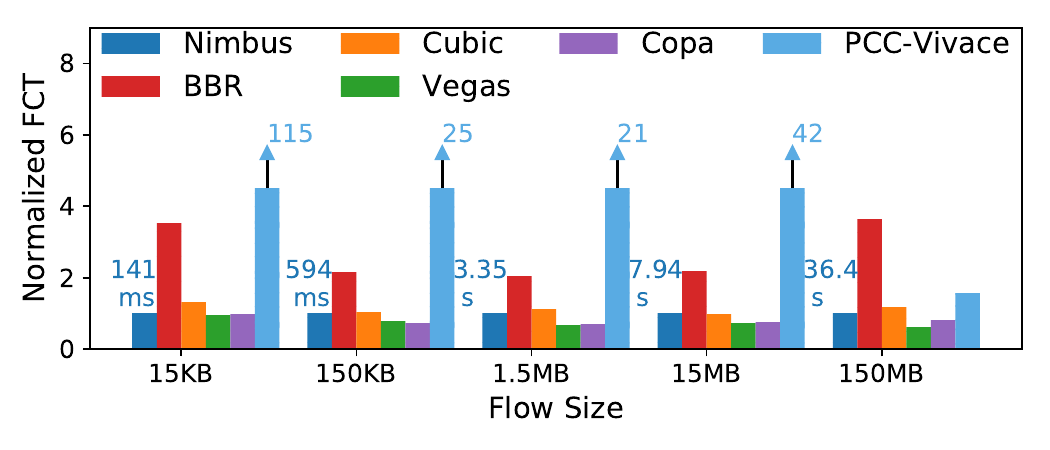}
    \caption{\small{Using \name reduces the p95 FCT of cross-flows relative to BBR at all flow sizes, and relative to Cubic for short flows. Vegas provides low cross-flow FCT, but its own rate is low.}}
    \label{fig:emp:fct}
\end{figure}

Using the same setup as \Sec{rw-wl}, we measure the flow completion time (FCT) of cross-flows.
\Fig{emp:fct} compares the 95th percentile (p95) cross-flow FCT for cross-flows of different sizes. The FCTs are normalized by the corresponding value for \name at each flow size.

BBR and PCC-Vivace exhibits much higher cross-flow FCT at all sizes compared to all the other protocols, consistent with the observation of unfairness ($\S$\ref{s:big-experiment}). 

For small cross-flows ($\leq$ 15 KB), the p95 FCT with \name and Copa are comparable to Vegas and lower than Cubic.
%
%For large cross-flows (150 MB or more), \name shares throughput fairly, giving tail FCT much smaller than BBR, which aggressively utilizes the link capacity.
%
With \name p95 FCT of cross traffic at higher flow sizes are slightly lower than Cubic because of small delays in switching to TCP-competitive-mode.
At all flow sizes, Vegas provides the best cross-flow FCTs, but its own flow rate is dismal; Copa is more aggressive than Vegas but less than Nimbus, but at the expense of its own throughput  (\Sec{rw-wl}).

\section{How Well Does \name Compete with BBR?}
\label{app:bbr-comparison}
\begin{figure}[tbh]
    \includegraphics[width=\columnwidth]{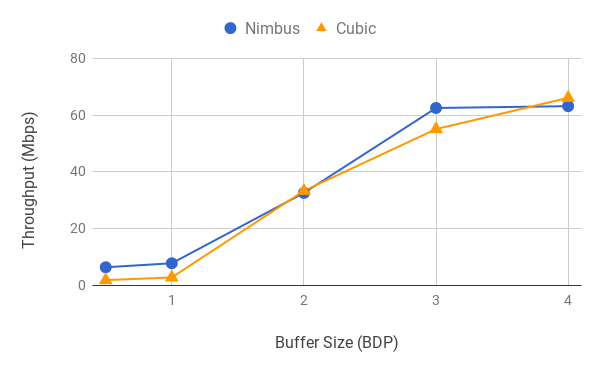}
    \vspace{-8mm}
    \caption{\textbf{ \name's performance against BBR is similar to that of Cubic.} Both \name and Cubic compete against 1 BBR flow on a 96 Mbit/s link. For various buffer sizes, \name achieves the same throughput as Cubic. }
    \label{fig:nimbus_vs_bbr}
\end{figure}
We now evaluate how well a \name (Cubic + BasicDelay) flow  competes with a BBR flow. 
In this experiment, the cross traffic is 1 BBR flow and the bottleneck link bandwidth is 96 Mbit/s. We vary the buffer size from 0.5 BDP to 4 BDP. \Fig{emp:switch} shows the average throughput of \name and Cubic flows while competing with BBR over a 2-minute experiment. \name achieves the same throughput as Cubic for all buffer sizes.

When the buffer size is $\leq$ 1 BDP, BBR is not ACK-clocked, and the elasticity detector classifies it as inelastic traffic. As a result, \name gets a relatively small fraction of the link bandwidth. In this scenario, Cubic also gets a small fraction of the link, because BBR sends traffic at its estimate of bottleneck link and is too aggressive. 

%rate and kills Cubic in the process.

When the buffer size is $\geq$ 1 BDP, BBR becomes ACK-clocked because of the cap on its congestion window. The elasticity detector now classifies BBR as elastic traffic. \name stays in competitive mode, behaving like Cubic and achieving the same throughput as Cubic.

\begin{figure}
    \centering
    \begin{subfigure}[b]{0.235\textwidth}
        \includegraphics[width=\textwidth]{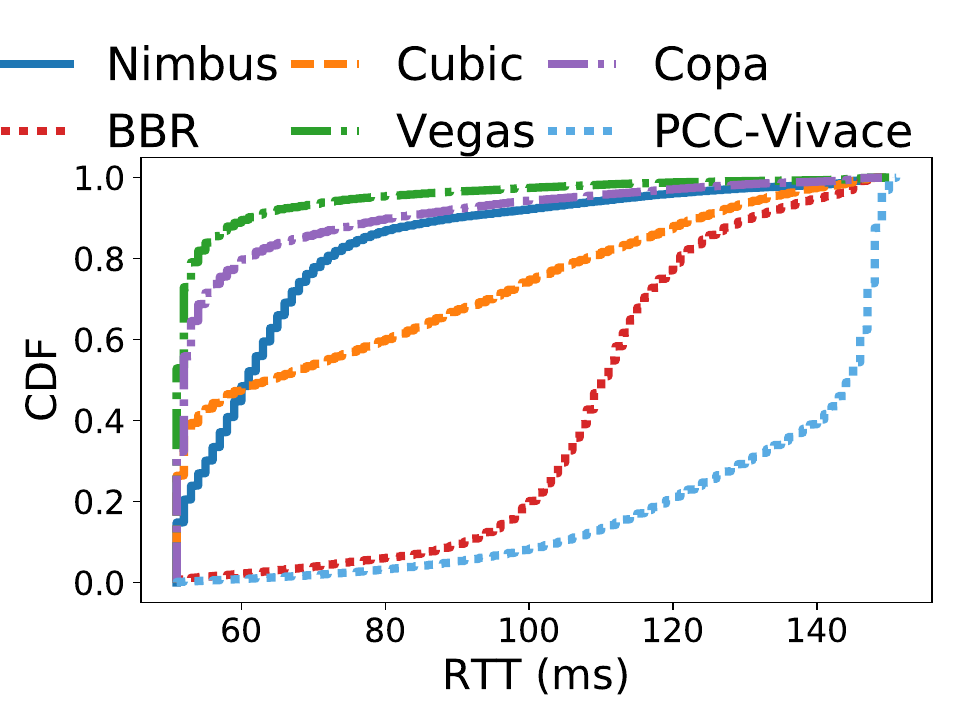}
        \vspace{-6mm}
        %\caption{\small{RTT}}
        \label{fig:emp_bbr:rtt}
    \end{subfigure}
    \begin{subfigure}[b]{0.235\textwidth}
        \includegraphics[width=\textwidth]{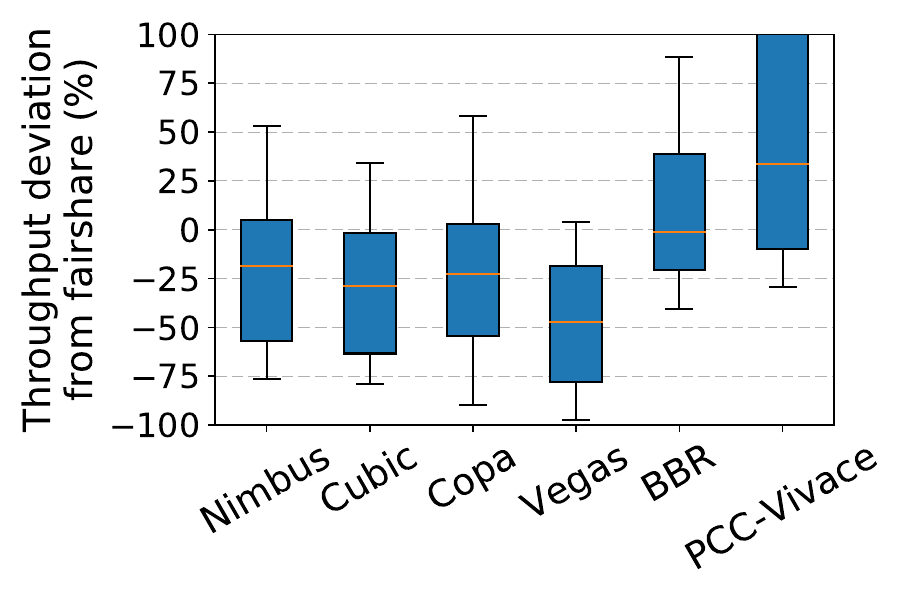}
        \vspace{-6mm}
        %\caption{\small{Deviation from fairshare}}
        \label{fig:emp_bbr:box}
    \end{subfigure}
    \vspace{-5mm}
    \caption{\small{{\bf WAN cross-traffic.} Cross traffic flows are running BBR. The deviation profile of \name{} is similar to that of Cubic, however, \name{} reduce delays significantly.}}
    \label{fig:emp_bbr}
    \vspace{-4mm}
\end{figure}
\smallskip
\noindent\textbf{WAN-cross traffic:}
We repeated the experiment in \Fig{big}, with cross traffic flows running BBR. \name is running Cubic in the TCP-competitive mode and BasicDelay in the delay-controlling mode. \Fig{emp_bbr} illustrates the performance of the various schemes. \name{}'s deviation profile is similar to that of Cubic, but \name{} achieves lower delays. However, both \name{} and Cubic achieve lower throughput than the fairshare, this is because Cubic doesn't compete will with BBR cross traffic. Copa and Vegas have similar delays as \name{}, but achieve lower throughput at the tail. PCC-Vivace is unfair to the cross traffic, and sends more than its fair-share.

\section{Understanding Scenarios where Copa's Mode Switching Makes Errors}
\label{app:copa-compare}

We explore the dynamics of our elasticity detector and Copa's mode switching in a few experiments from the scenarios described in $\S$\ref{s:copa-compare}. Recall that the link capacity is 96 Mbit/s, the propagation RTT is 50~ms, and the buffer size is 2~BDP.

\subsection{Constant Bit Rate Cross Traffic}
\Fig{appendix-cbr} shows throughput and delay profile for Copa and \name while competing against inelastic Constant Bit Rate (CBR) traffic. We consider two scenarios: (i) CBR occupies a small fraction of the link (24 Mbits/s, 25\%) and (ii) CBR occupies majority of the link (80 Mbit/s, 83\%). 
When the CBR traffic is low (\Fig{appendix-cbr} \subref{fig:appendix-cbr:copa-24} and \subref{fig:appendix-cbr:nimbus-24}), both Copa and the elasticity detector identify it as non buffer-filling and inelastic respectively and achieve low queuing delays.

When the CBR's share of the link is high (\Fig{appendix-cbr} \subref{fig:appendix-cbr:copa-80}), Copa incorrectly classifies the cross traffic as buffer-filling and as a result stays in competitive mode, leading to high queuing delays. Copa relies on a pattern of emptying queues to detect whether the cross traffic is buffer-filling or not. However, when the rate of cross traffic is $z$, the fastest possible rate at which the queue can drain is $\mu - z$, even if Copa reduces its rate to zero. If the cross traffic occupies $x$ fraction of the link (\ie $z = x \cdot \mu$, then:
\begin{align}
    \max(-\frac{dQ}{dt}) &= \mu - z \\ \nonumber
                        &= (1 - x) \times \mu\\ \nonumber
                        &= (1 - x) \times \frac{BDP}{RTT}. \nonumber
\end{align}
Therefore, if the queue size ever exceeds $5 \times  (1 - x) BDP$, then Copa won't be able to drain the queue in 5 RTTs, and it will mis-classify the cross traffic as buffer-filling. The queue size can grow large due to a transient burst or if Copa incorrectly switches to competitive mode. Once Copa is in competitive mode, it will drive the queues even higher and can therefore get stuck in competitive mode.

In contrast (\Fig{appendix-cbr} \subref{fig:appendix-cbr:nimbus-80}), our detector doesn't rely on emptying queues and correctly classifies cross traffic as inelastic, achieving low queuing delays.
\begin{figure}[tbh]
    \begin{center}
        \begin{subfigure}[b]{\columnwidth}
            \includegraphics[height=1.35in,width=0.8\columnwidth]{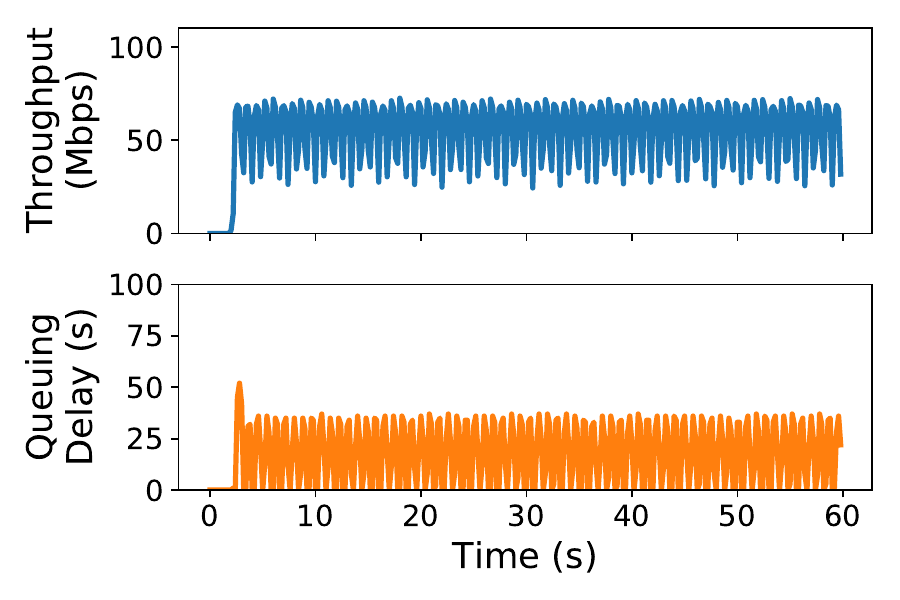}
            \vspace{-3mm}
            \subcaption{Copa: 24 Mbit/s CBR}
            \label{fig:appendix-cbr:copa-24}
        \end{subfigure}
        \begin{subfigure}[b]{\columnwidth}
            \includegraphics[height=1.35in,width=0.8\columnwidth]{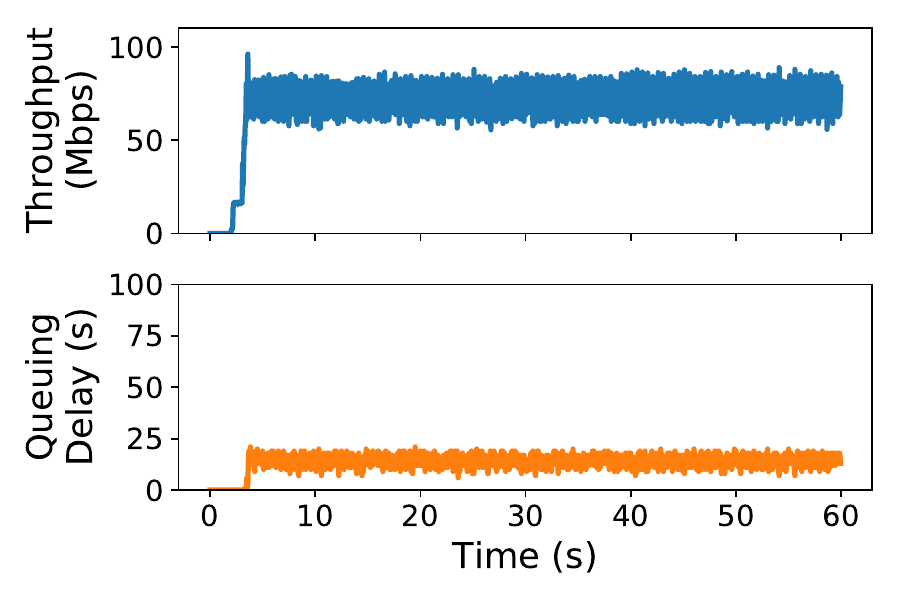}
            \vspace{-3mm}
            \subcaption{\name: 24 Mbit/s CBR}
            \label{fig:appendix-cbr:nimbus-24}
        \end{subfigure}
        \begin{subfigure}[b]{\columnwidth}
            \includegraphics[height=1.35in,width=0.8\columnwidth]{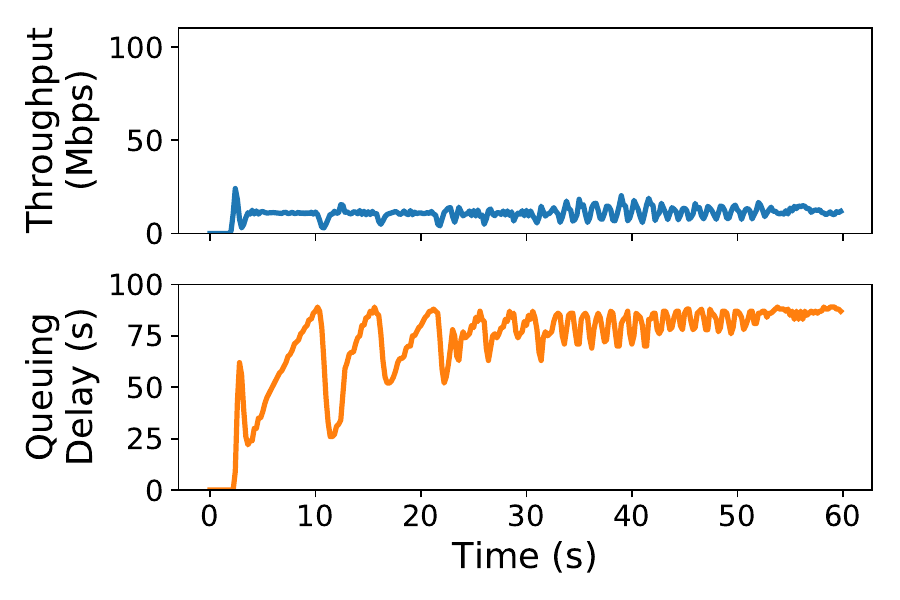}
            \vspace{-3mm}
            \subcaption{Copa: 80 Mbit/s CBR}
            \label{fig:appendix-cbr:copa-80}
        \end{subfigure}
        \begin{subfigure}[b]{\columnwidth}
            \includegraphics[height=1.35in,width=0.8\columnwidth]{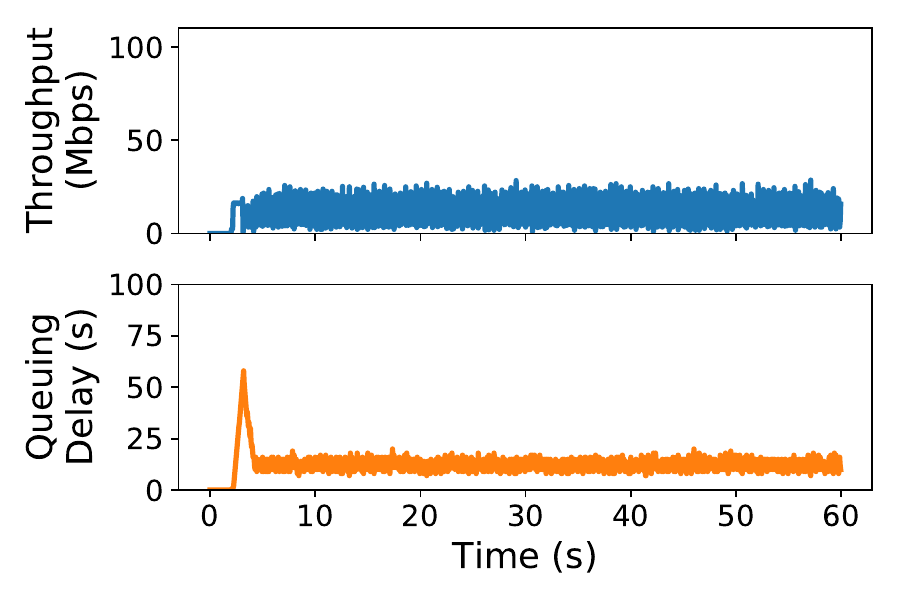}
            \vspace{-3mm}
            \subcaption{\name: 80 Mbit/s CBR}
            \label{fig:appendix-cbr:nimbus-80}
        \end{subfigure}
        \caption{\textbf{Queuing delay and throughput dynamics for inelastic CBR cross traffic.} When the CBR traffic is low (\subref{fig:appendix-cbr:copa-24}), Copa classifies the traffic as non buffer-filling and is able to achieve low queuing delays. But when the CBR traffic occupies a high fraction (\subref{fig:appendix-cbr:copa-80}), Copa incorrectly classifies the traffic as buffer-filling, resulting in higher queuing delays. In both the situations (\subref{fig:appendix-cbr:nimbus-24} and \subref{fig:appendix-cbr:nimbus-80}), our elasticity detector correctly classifies the traffic as inelastic and \name achieves low queuing delays.}
        \label{fig:appendix-cbr}
    \end{center}
\end{figure}

\subsection{Elastic cross traffic}
\Fig{appendix-cross} shows throughput and delay over time for Copa and \name while competing against an elastic NewReno flow. We consider two scenarios: (1) both flows have the same propagation RTT, and (2) the cross traffic's propagation RTT is $4\times$ higher than the Copa or \name flow. When the RTTs are the same (\Fig{appendix-cross} \subref{fig:appendix-cross:copa-1} and \subref{fig:appendix-cross:nimbus-1}), both Copa and our elasticity detector correctly classify the cross traffic, achieving a fair share of throughput.

When the cross traffic RTT is higher (\Fig{appendix-cross} \subref{fig:appendix-cross:copa-4}), the NewReno flow ramps up its rate slowly, causing Copa to mis-classify the traffic and achieve less than its fair share of the throughput. Here, Copa achieves 27 Mbit/s but its fair share is at least 48 Mbit/s (and 77 Mbit/s if one considers the RTT bias). In contrast (\Fig{appendix-cross} \subref{fig:appendix-cross:nimbus-4}), our elasticity detector correctly classifies the cross traffic as elastic, and \name achieves its RTT-biased share of throughput.

\begin{figure}
    \begin{center}
        \begin{subfigure}{\columnwidth}
            \includegraphics[height=1.35in,width=0.8\columnwidth]{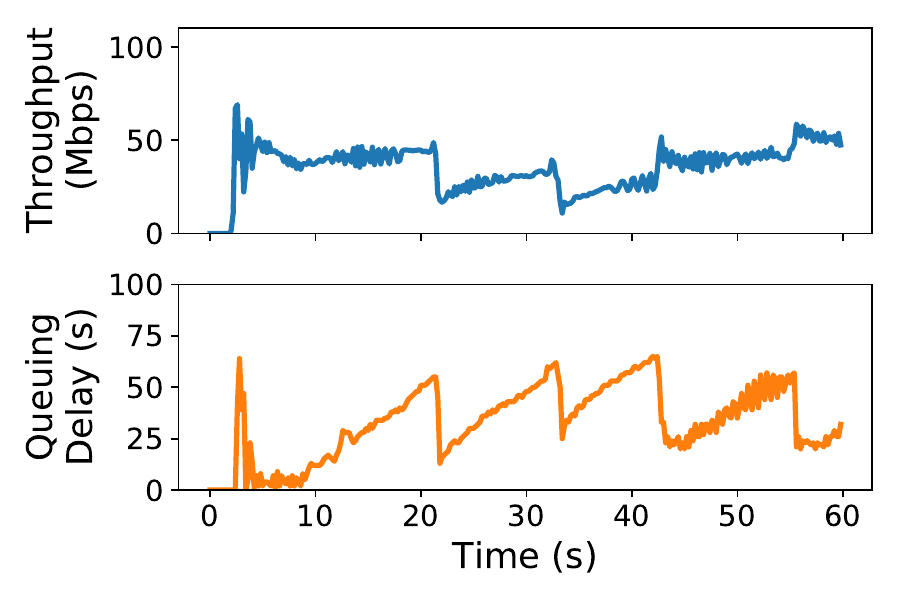}
            \vspace{-3mm}
            \subcaption{Copa: Cross Traffic RTT = 1 $\times$ Flow RTT}
            \label{fig:appendix-cross:copa-1}
        \end{subfigure}
        \begin{subfigure}{\columnwidth}
            \includegraphics[height=1.35in,width=0.8\columnwidth]{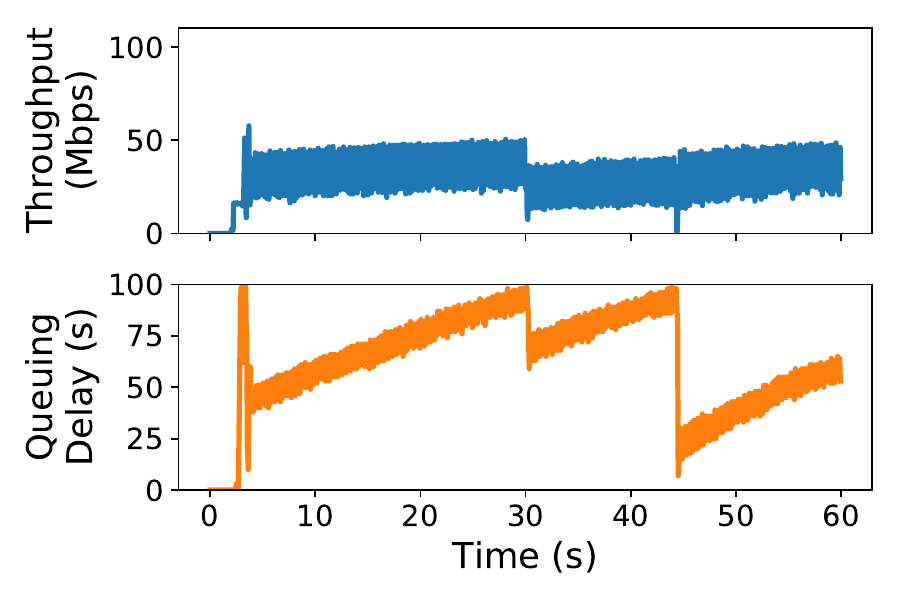}
            \vspace{-3mm}
            \subcaption{\name: Cross Traffic RTT = 1 $\times$ Flow RTT}
            \label{fig:appendix-cross:nimbus-1}
        \end{subfigure}
        \begin{subfigure}{\columnwidth}
            \includegraphics[height=1.35in,width=0.8\columnwidth]{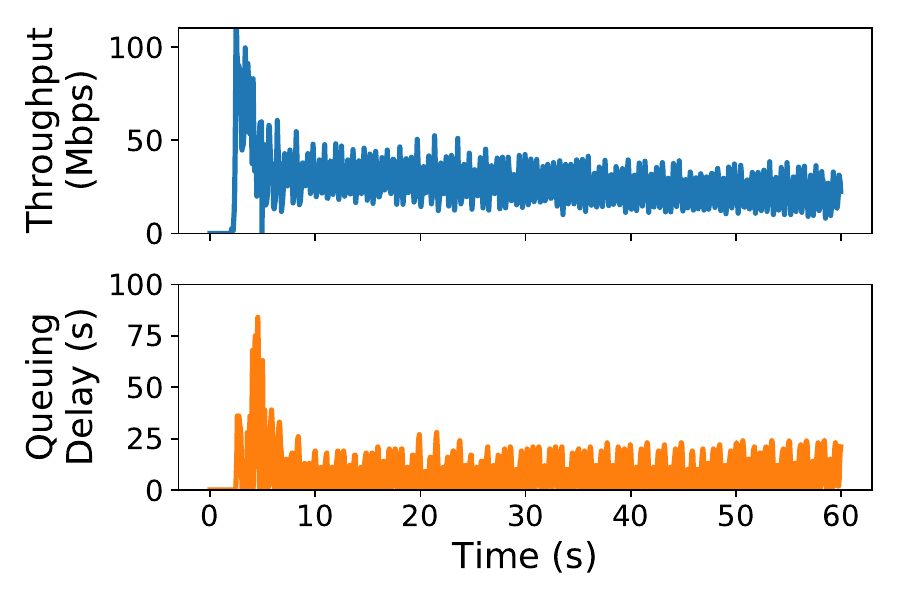}
            \vspace{-3mm}
            \subcaption{Copa: Cross Traffic RTT = 4 $\times$ Flow RTT}
            \label{fig:appendix-cross:copa-4}
        \end{subfigure}
        \begin{subfigure}{\columnwidth}
            \includegraphics[height=1.35in,width=0.8\columnwidth]{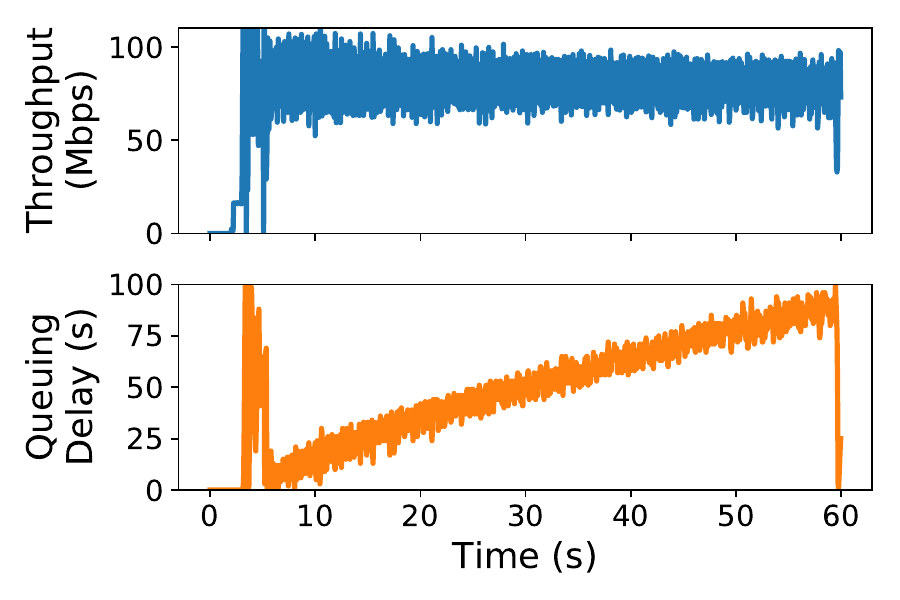}
            \vspace{-3mm}
            \subcaption{\name: Cross Traffic RTT = 4 $\times$ Flow RTT}
            \label{fig:appendix-cross:nimbus-4}
        \end{subfigure}
        \caption{\textbf{Queuing delay and throughput dynamics for elastic cross traffic.} When the elastic cross traffic increases fast enough (\subref{fig:appendix-cross:copa-1}), Copa classifies it as buffer-filling and is able to achieve its fair share. But, when the elastic cross traffic increases slowly (\subref{fig:appendix-cross:copa-4}), Copa incorrectly classifies the traffic as non buffer-filling, achieving less throughput than its fair share. In both the situations (\subref{fig:appendix-cross:nimbus-1} and \subref{fig:appendix-cross:nimbus-4}), our elasticity detector correctly classifies the traffic as elastic and \name is able to achieve its fair share of throughput. }
        \label{fig:appendix-cross}
    \end{center}
\end{figure}

%\section{Robustness of elasticity detection: multi-factor experiments}
%\label{app:robustness-multifactor}

\if 0
\subsection{Pulse size, link rate, and offered link load}
We perform a multi-factor experiment varying \possname pulse size, link rate, and link share as described in \Sec{multifactor-robustness-first-half}.

\Fig{heatmap} shows the average detection accuracy over five runs of the other two categories of cross-traffic (mix + purely inelastic).
\name achieves an accuracy of more than 90\% averaged over all the points.
In general, increasing the pulse sizes improves accuracy because \name can create a more easily observable change in the cross-traffic sending rates.
An increase in the link rate results in higher accuracy for a given pulse size and \name link share because the variance in the rates of inelastic Poisson cross-traffic reduces with increasing cross-traffic sending rate, reducing the number of false peaks in the cross-traffic FFT.
For the same reason, decreasing \possname share of the link also results in higher accuracy in general.
However, at low link rates, \name has low accuracy ($\sim$60\%) when it uses high pulse sizes and controls a low fraction of the link rate. We believe that this is due to a quirk in the way the Linux networking stack reports round-trip time measurements under sudden sending rate changes.

\begin{figure}
    \includegraphics[width=\columnwidth]{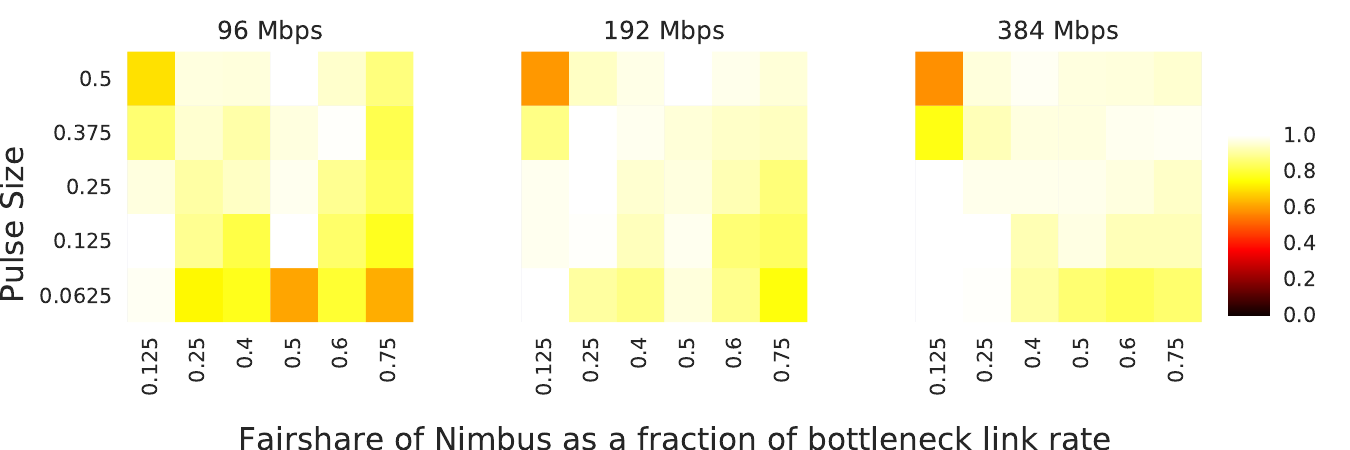}
    \vspace{-6mm}
    \caption{\small \name is robust to variations in link bandwidth and fraction of traffic controlled by it. Increasing pulse size increases robustness.}
    \label{fig:heatmap}
    \vspace{-4mm}
\end{figure}
\fi 
\section{Buffer size, RTT, and AQM}
\label{app:robustness:bufsize-rtt-aqm}
We vary the bottleneck buffer size (drop-tail) from 0.25 BDP to 4 BDP for three categories of cross traffic as in the earlier experiments, with propagation delays of 25 ms, 50 ms, and 75 ms. We also measured classification accuracy when the bottleneck link implements PIE~\cite{pie} at two target delays (0.25 BDP and 1 BDP) with a propagation delay of 50 ms.
With purely elastic or inelastic traffic, the elasticity detector has an average accuracy (across 5 runs) of 98\% or more in all cases but two, while with mixed traffic, the accuracy is always 85\% or more.
In all cases (including low accuracy ones), \name achieves its fair-share throughput and low delays.

Now we discuss the cases with low classification accuracy.
First, with shallow buffers of size less than the product of the delay threshold $x_{t}$ and the bottleneck link rate (\eg 0.25 BDP when the \rtt is 50 ms), the elasticity detector classifies all traffic as elastic. Second, with the bottleneck link implementing PIE with small target delay (\eg corresponding to 0.25 BDP), the elasticity detector classifies all traffic as elastic. In both cases, \name can incur heavy losses in delay-control mode as \name's target queuing delay of 0.25 BDP is comparable to the drop-tail buffer size or target delay of PIE. 
These losses interfere with the cross-traffic estimator leading to classification errors (in delay-control mode). However, low accuracy does not impact the performance of \name as it achieves its fair-share throughput and low delays (bounded by the small buffer size for a drop-tail queue and the delay control threshold of PIE).
Further, classification accuracy decreases when \possname RTT exceeds its pulse period. Since \possname measurements of rates are over one RTT, any oscillations over a smaller period cannot be observed.

%
% Our results were similar when the propagation delay was 25ms and 75ms.

\cut{
\begin{figure}
    \includegraphics[width=0.8\columnwidth]{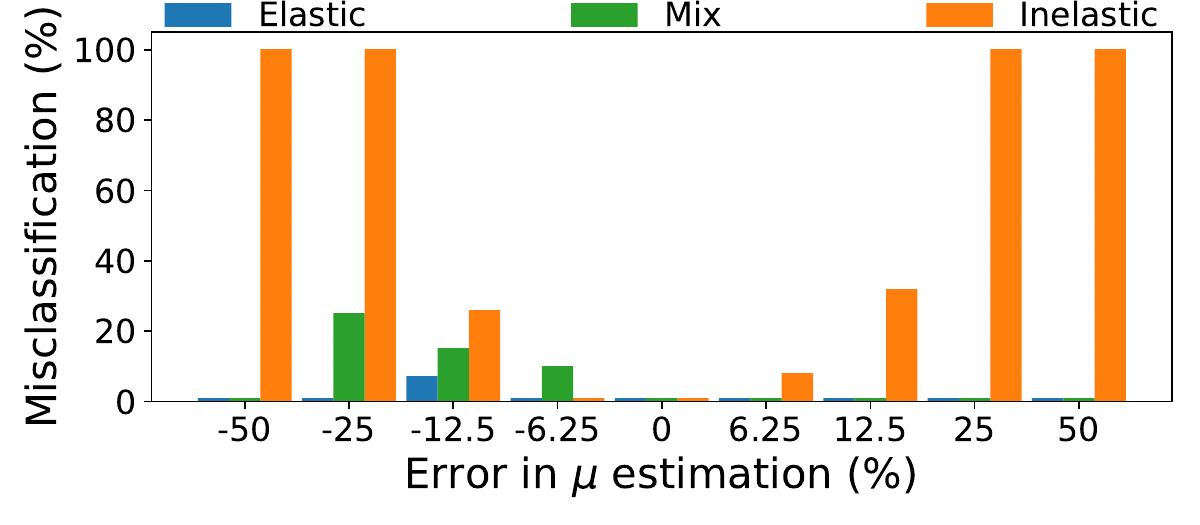}
    \vspace{-6mm}
    \caption{\small Impact of error in link rate estimation on classification accuracy. Classification accuracy for elastic and mix (elastic + inelastic) traffic remains high. When the error is high, all traffic is classified as elastic.}
    \label{fig:bandwidth_error}
    \vspace{-4mm}
\end{figure}
\subsection{Inaccuracies in link rate estimation}
\label{app:robustness:bad-mu}
We evaluate the impact of inaccuracies in link rate estimation on the classification accuracy. We vary the link rate estimate from -50\% to +50\% of the real link rate value. \Fig{bandwidth_error} shows the mis-classification rate for different error rates. The classification accuracy is high for all traffic classes when the error is less than equal to 12.5\%. When the error rate is higher (>= 25\%), all cross traffic is classified as elastic. 

The explanation is as follows. Let's define $\hat{z}(t)$ as our estimate of the cross traffic rate, $z^{*}(t)$ as the real cross traffic rate, $\hat{\mu}$ as our estimate of the link rate and $\mu^{*}$ as the real link rate. Then, from Equation ~\ref{eq:zfromR}, we get
\begin{align}
    \hat{z}(t) &= \hat{\mu} \frac{S(t)}{R(t)} - S(t) \\ \nonumber
      z^{*}(t) &= \mu^{*} \frac{S(t)}{R(t)} - S(t) \nonumber
\end{align}
Combining the equations above, we get
\begin{align}
    \hat{z}(t) &= \frac{\hat{\mu}}{\mu^{*}} z^{*}(t) + \big(\frac{\hat{\mu}}{\mu^{*}} - 1 \big) S(t)  \\ \nonumber
\end{align}

When the link estimate is incorrect, the cross traffic estimate is a linear combination of the real cross traffic rate and the sending rate. As the error increases, the contribution of the sending rate to the cross traffic estimate increases. Since the sending rate oscillates at the pulse frequency, the cross traffic estimate oscillates, and all the cross traffic (regardless of it's nature) is classified as elastic.

For \name{} this implies that when the error in link rate estimate is high, it uses the TCP-competetive mode regardless of the nature of the cross traffic. In this case, against inelastic cross traffic, \name loses the benefits of delay-controlling mode. However, by always running in TCP-competetive mode, Nimbus doesn't lose throughput due to inaccuracies in link rate estimation. Thus, Nimbus is safe under such inaccuracies.
}
\section{Detecting non-ACK-Clocked \\ Elastic Cross Traffic}
\label{app:slow-react}
\begin{figure}
    \centering
    \includegraphics[width=0.9\columnwidth]{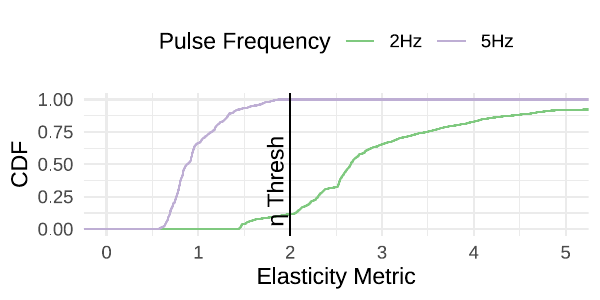}
    \caption{\small By modifying the Nimbus pulse frequency, the detector will classify PCC Vivace, a rate based protocol, as elastic.}
    \label{fig:vivace-elastic}
\end{figure}

Recall that by default our elasticity detector aims to detect ACK-clocked elastic flows that react quickly to changes in available bandwidth on RTT timescales. This experiment demonstrates our elasticity detector's ability to also detect slow-reacting elastic cross traffic by tuning the pulse frequency. 
We ran a \name flow against a PCC-Vivace flow on a 96Mbit/s link with 100ms of buffering. 
\Fig{vivace-elastic} shows that CDF of elasticity metric for 2 different pulse frequencies ($f_{p}$). 
PCC-Vivace is not ACK-clocked and does not react to the elasticity detector's pulses at 5Hz. 
As a result the elasticity metric, $\eta$, is below the threshold most of the time. 
Reducing the pulse frequency to 2Hz creates pulses with a longer duration. 
PCC-Vivace reacts to these slower variations in available bandwidth and is thus correctly classified as elastic ($\eta$ > $\eta_{Thresh}$). 

Changing the pulse frequency involves a trade-off. 
Increasing the pulse duration might temporarily increase queuing delays, hurting performance. 
Since most of the elastic traffic is ACK-clocked and hence fast reacting, we propose using a small pulse duration (e.g., 200ms). 
In the future, if slowly-reacting protocols become widely deployed,
%In the future, if the slowly-reacting elastic cross traffic is widely deployed, 
the elasticity detector could be configured accordingly by adjusting the pulse duration.
