# Supplementary material for: Elasticity Detection: A Building Block for Internet Congestion Control
Source: arXiv:1802.08730 source file (2020-02-15)
Supplement: Supplementary file 5 [file load-var-appendix.tex]

\newpage

\newpage

\section{Impact of varying cross traffic load}
\label{app:load-var}

\Fig{load-var1} shows that as the cross traffic' load increases \name's RTTs increase.

Table~\ref{tab:var-load2} shows the impact of cross traffic load on \name's switching mechanism. When the cross traffic load is low ($<20\%$) or high ($>80\%$) \name's classification error is low and we see that ground traffic (percentage of elastic cross traffic to link capacity) remains pretty much the same throughout. For load's between (20 and 80 percent) switching happens quite often. Under these conditions \name make a classification error of 25\%.

\begin{table}
\begin{center}
 \begin{tabular}{||c c||} 
 Cross Traffic Load(\%) & Miss-classification (\%)\\
 10 & 9.6\\ 
 30 & 28.4\\ 
 50 & 24.1\\ 
 70 & 26.3\\ 
 90 & 14.9
\end{tabular}
\end{center}
\caption{\small {\bf Elasticity miss-classification vs. cross traffic load---}The elasticity estimation becomes more accurate with both low and high cross traffic load.} 
\label{tab:var-load2}
\end{table}

\begin{figure}[h]
\centering
    \includegraphics[width=0.8\columnwidth]{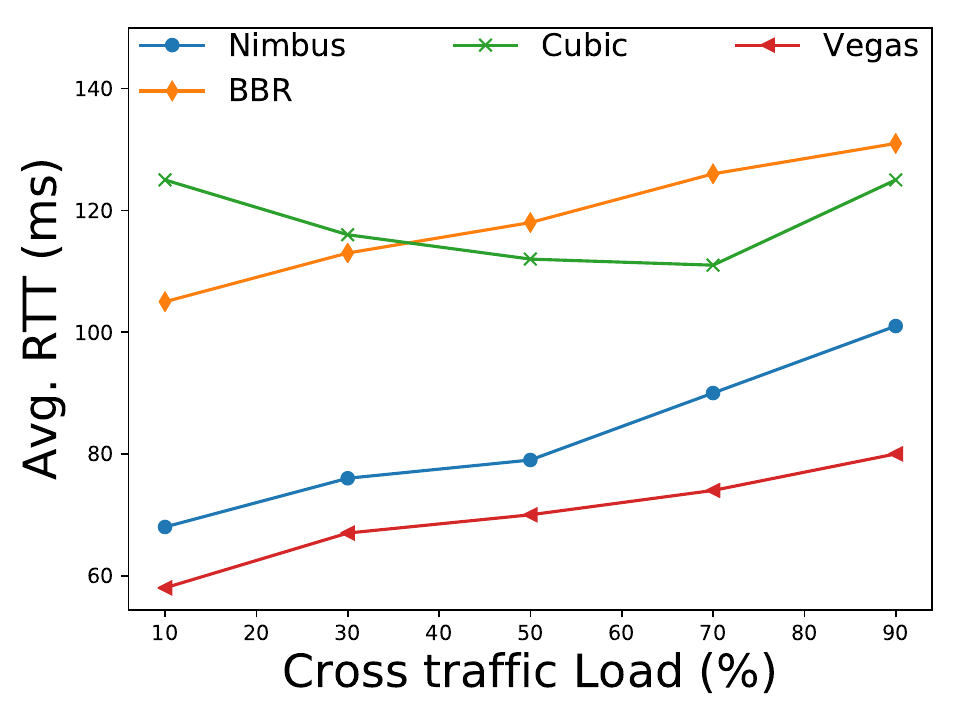}
    \caption{\small {\bf Average RTT vs. cross traffic load---}\name reduces delays more effectively at low cross traffic load.}
    \label{fig:load-var1}
\end{figure}
